# Supplementary material for: CarPlanner: Consistent Auto-regressive Trajectory Planning for Large-scale Reinforcement Learning in Autonomous Driving
Source: arXiv:2502.19908 source file (2025-03-24)
Supplement: Supplementary file 1 [file table_supple_rl_horizon.tex]

\begin{table}[t]
    % \vspace{6pt}
    \centering
    % \vspace{-0.2cm}
    \setlength{\tabcolsep}{3pt} % Adjust the space between columns
    \setlength{\aboverulesep}{0.3pt}
    \setlength{\belowrulesep}{0.3pt}
    % \small
    \fontsize{5pt}{6pt}\selectfont % Set font size and line spacing
    \resizebox{0.49\textwidth}{!}{\begin{tabular}{c | c |  c c c c c  }
    \toprule
    \multicolumn{2}{c|}{Time horizon} & \multicolumn{5}{c}{Closed-loop metrics ($\uparrow$)}  \\
    \midrule
    Train & \makecell{Test} &  CLS-NR &  S-CR  & S-Area  & S-PR & S-Comfort   \\
    \midrule
    \multirow{4}{*}{\makecell{1}} 
            & 1     &  75.79 & 87.18  & 88.89  & 90.99  & 87.18   \\ 
            & 3     &  73.04 & 86.70  & 92.66  & 86.33  & 63.30   \\ 
            & 5     &  71.55 & 85.91  & 91.82  & 85.69  & 60.91   \\ 
            & 8     &  71.55 & 85.91  & 91.82  & 85.69  & 60.91   \\ 
    \midrule
    \multirow{4}{*}{\makecell{3}} 
            & 1     &  86.08 & 95.95  & 97.68  & 85.70  & 84.17   \\ 
            & 3     &  88.65 & 97.10  & 97.68  & 87.96  & 92.66   \\ 
            & 5     &  89.39 & 97.31  & 98.46  & 88.04  & 86.54   \\ 
            & 8     &  89.36 & 97.31  & 98.46  & 87.93  & 86.54   \\ 
    \midrule
    \multirow{4}{*}{\makecell{5}} 
            & 1     &  85.09 & 95.56  & 96.53  & 89.92  & 89.58   \\ 
            & 3     &  91.14 & 96.73  & 98.85  & 91.95  & 91.54   \\ 
            & 5     &  91.72 & 97.69  & 98.85  & 92.58  & 90.77   \\ 
            & 8     &  91.80 & 98.08  & 98.85  & 92.55  & 90.38   \\ 
    \midrule
    \multirow{4}{*}{\makecell{8}} 
            & 1     &  87.43 & 94.98  & 98.46  & 91.13  & 90.73   \\ 
            & 3     &  93.93 & 98.84  & 98.84  & 94.97  & 91.86   \\ 
            & 5     &  93.94 & 99.22  & 99.22  & 95.04  & 91.09   \\ 
            & 8     &  94.07 & 99.22  & 99.22  & 95.06  & 91.09   \\ 
    \bottomrule
    \end{tabular}}
    % \vspace{-0.3cm}
    \caption{\red{todo}}
    \label{table:supple-abla-rl-horizon}
    % \vspace{-0.3cm}
\end{table}
